# Supplementary material for: Stable Ferromagnetism and High Curie Temperature in VGe$_2$N$_4$
Source: arXiv:2202.06424 source file (2022-05-05)
Supplement: Supplementary file 1 [file SI-20220419.pdf]

# Supporting Information

## Stable Ferromagnetism and High Curie Temperature in $VGe_2N_4$

Yingmei Li, Yong Liu*

*State Key Laboratory of Metastable Materials Science and Technology, Yanshan University, Qinhuangdao 066004, China*

E-mail: yongliu@ysu.edu.cn

Table S1 Magnetic anisotropy energy (MAE in meV, which is defined as $E_{[001]}$-$E_{[100]}$) for $VGe_2N_4$ under strain.

| Lattice b | MAE |
|---|---|
| 4.7 Å | -0.0078 |
| 4.8 Å | 0.0019 |
| 4.9 Å | 0.0014 |
| 5.0 Å | -0.0062 |
| 5.1 Å | -0.0003 |
| 5.2 Å | 0.0119 |
| 5.3 Å | -0.0068 |
| 5.4 Å | 0.0002 |
| 5.5 Å | -0.0061 |
| 5.6 Å | 0.0033 |
| 5.7 Å | -0.0078 |
| 5.8 Å | -0.0074 |

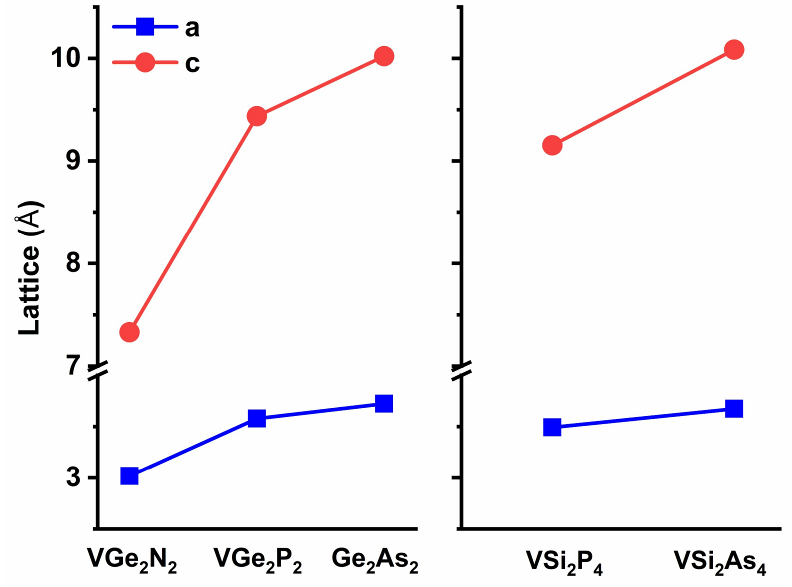


Fig. S1 Lattice parameters for $VGe_2N_4$, $VGe_2P_4$, $VGe_2As_4$, $VSi_2P_4$ and $VSi_2P_4$.

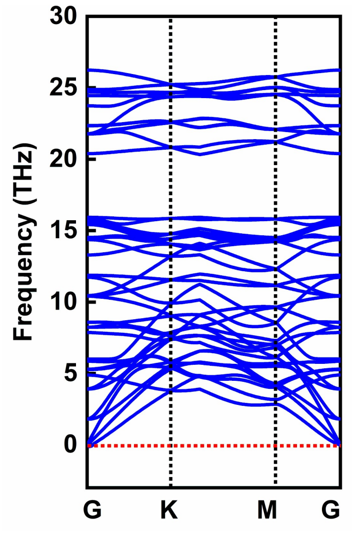


Fig. S2 Calculated phonon dispersion curves for $VGe_2N_4$.

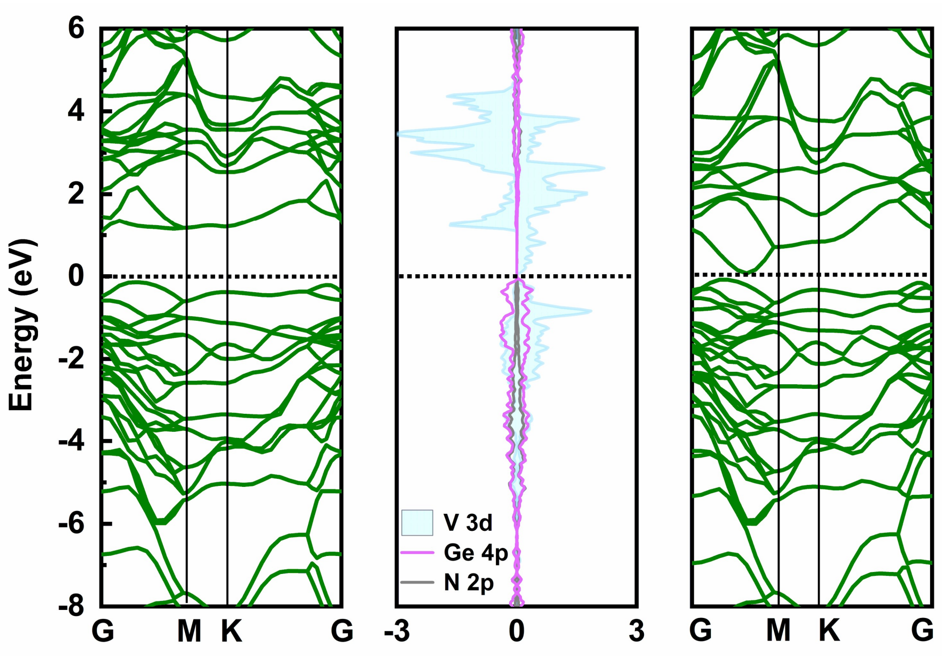


Fig. S3 Band structure and partial density of states for $VGe_2N_4$ with b = 5.8 Å.

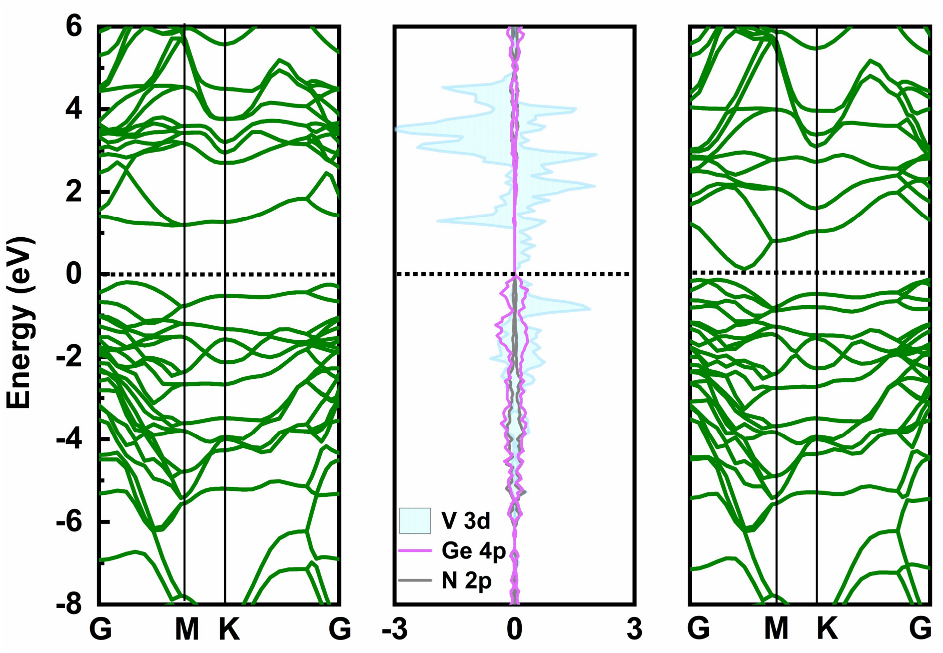


Fig. S4 Band structure and partial density of states for $VGe_2N_4$ with b = 5.7 Å.

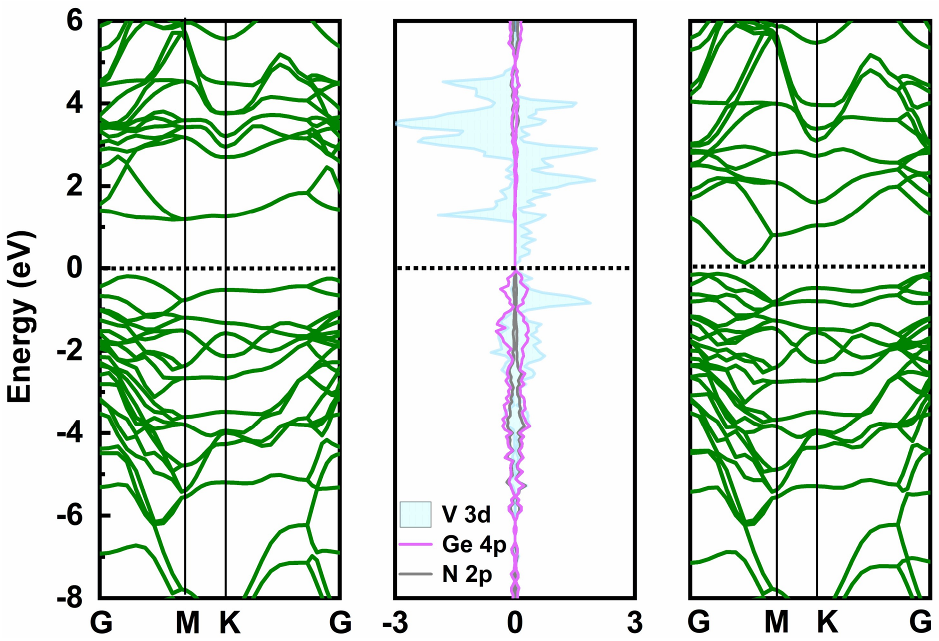


Fig. S5 Band structure and partial density of states for $VGe_2N_4$ with b = 5.6 Å.

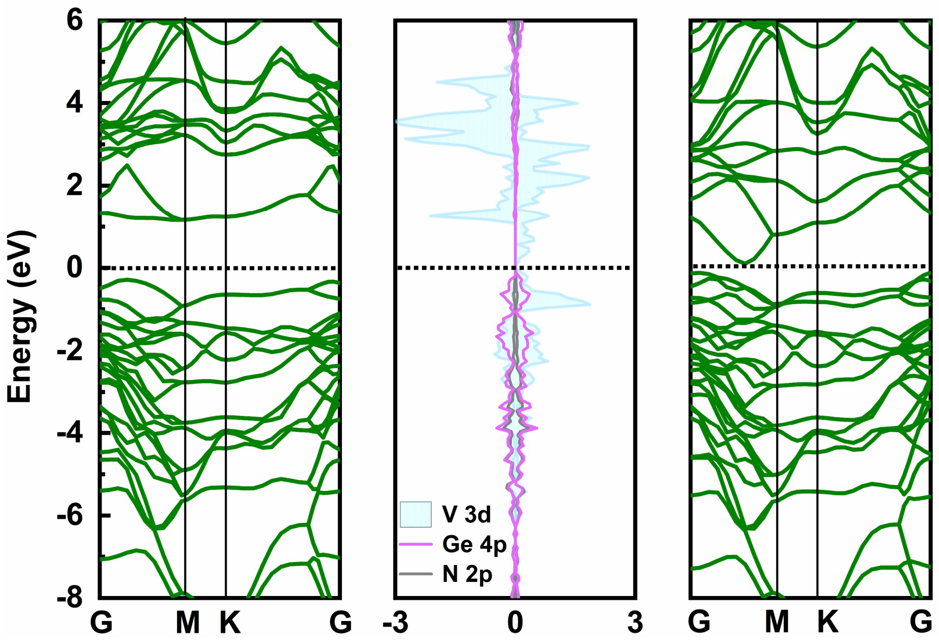


Fig. S6 Band structure and partial density of states for $VGe_2N_4$ with b = 5.5 Å.

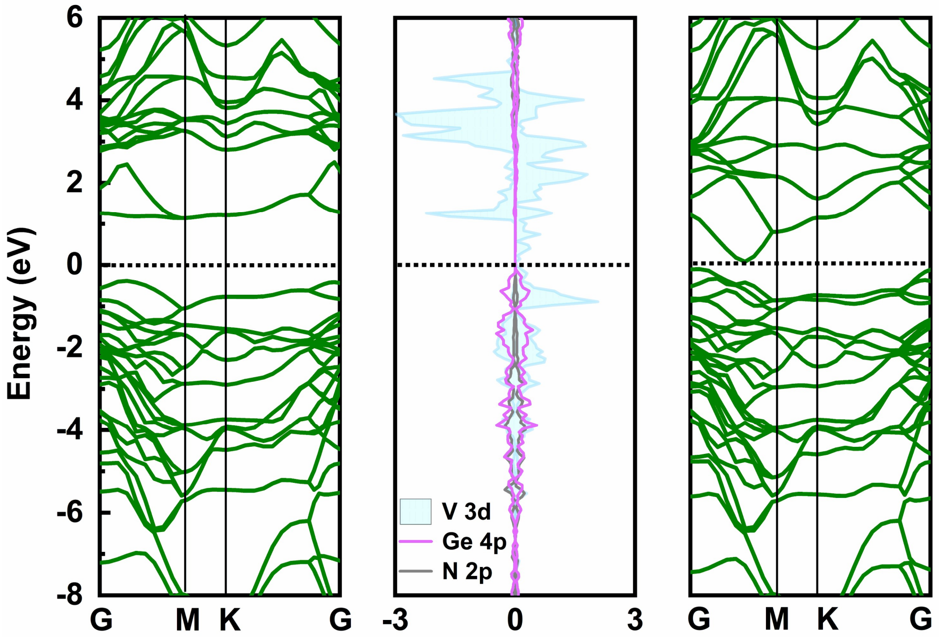


Fig. S7 Band structure and partial density of states for $VGe_2N_4$ with b = 5.4 Å.

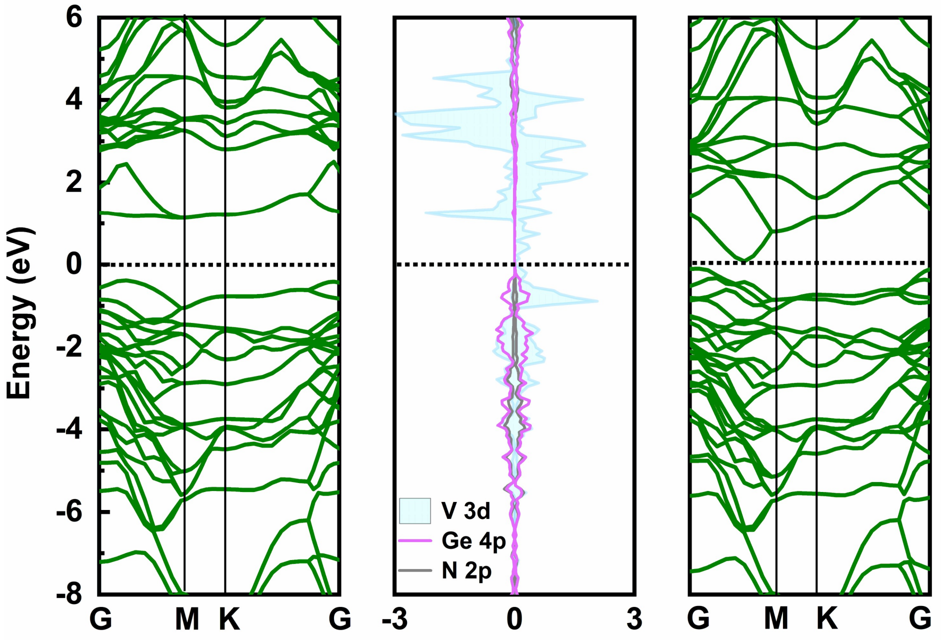


Fig. S8 Band structure and partial density of states for $VGe_2N_4$ with b = 5.3 Å.

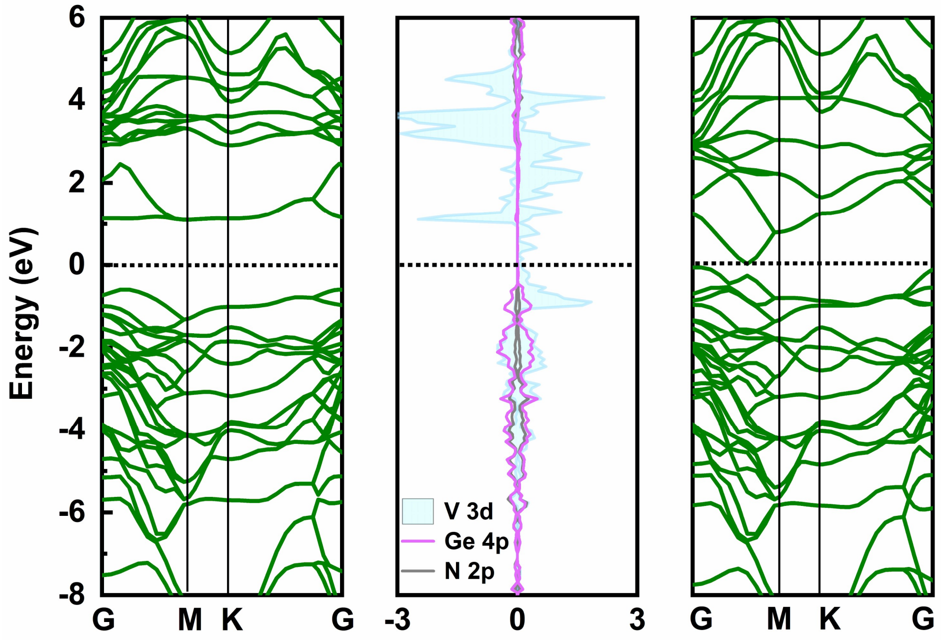


Fig. S9 Band structure and partial density of states for $VGe_2N_4$ with b = 5.2 Å.

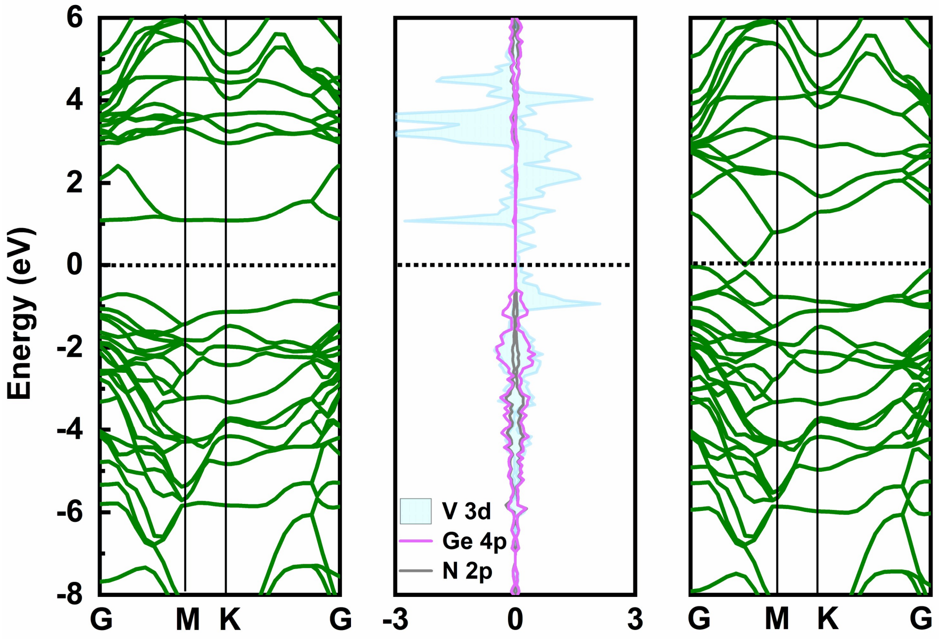


Fig. S10 Band structure and partial density of states for $VGe_2N_4$ with b = 5.1 Å.

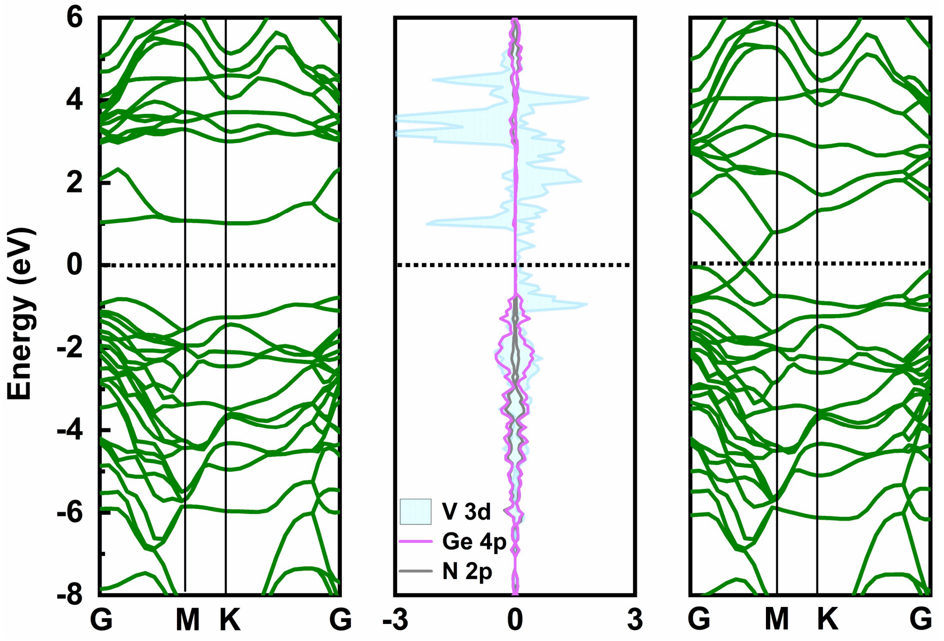


Fig. S11 Band structure and partial density of states for $VGe_2N_4$ with b = 5.0 Å.

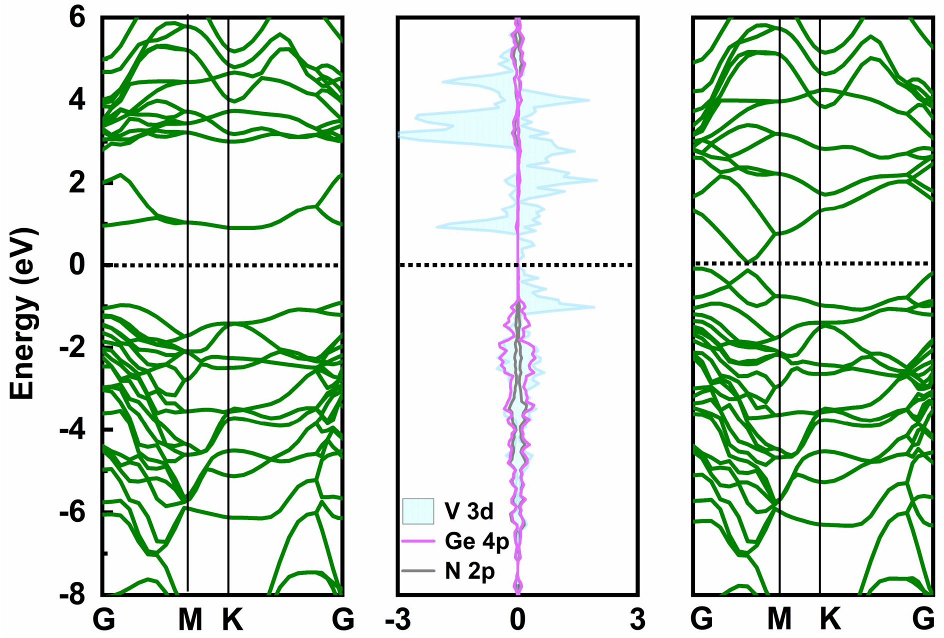


Fig. S12 Band structure and partial density of states for $VGe_2N_4$ with b = 4.9 Å.

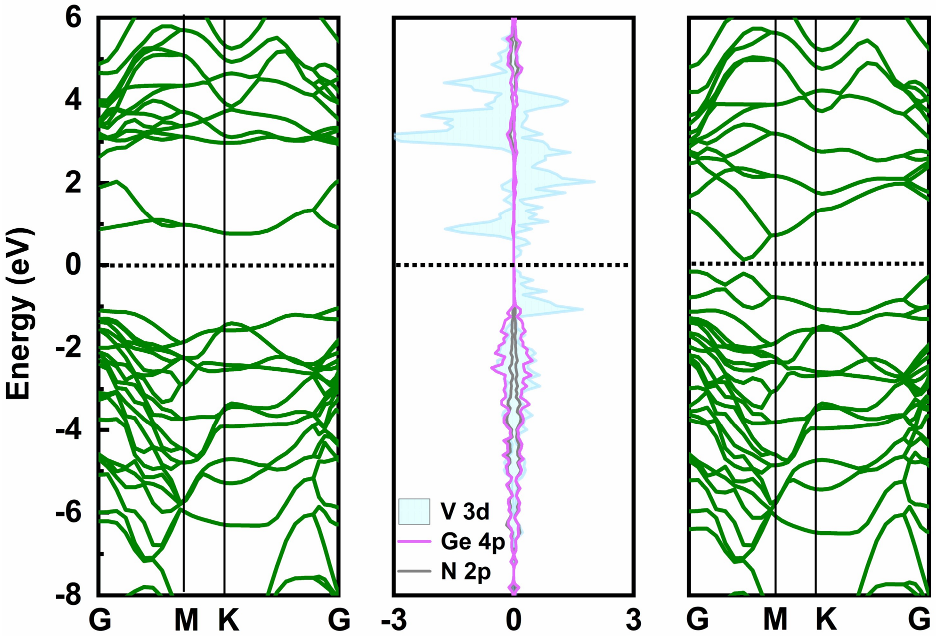


Fig. S13 Band structure and partial density of states for $VGe_2N_4$ with b = 4.8 Å.

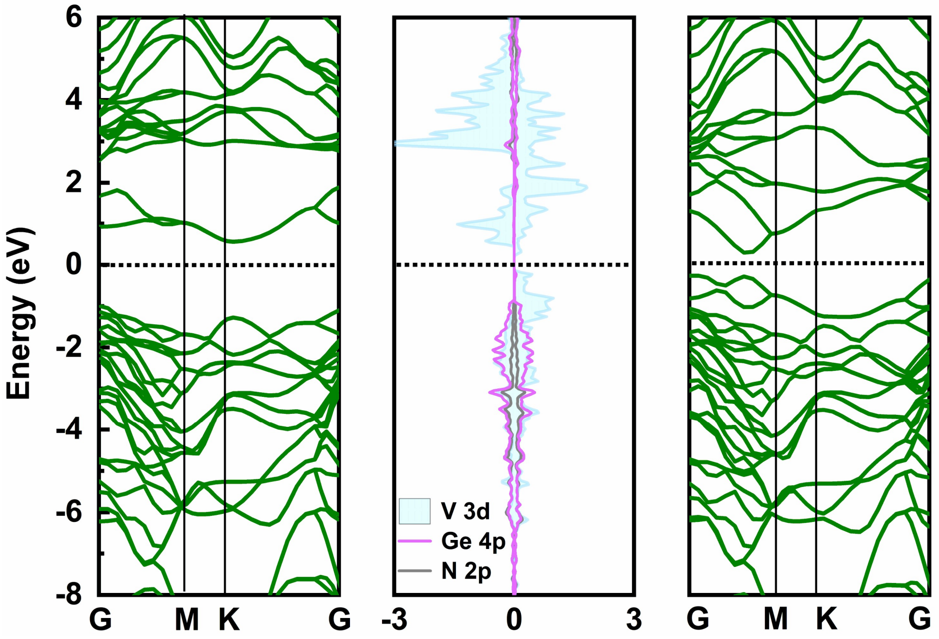


Fig. S14 Band structure and partial density of states for $VGe_2N_4$ with b = 4.7 Å.

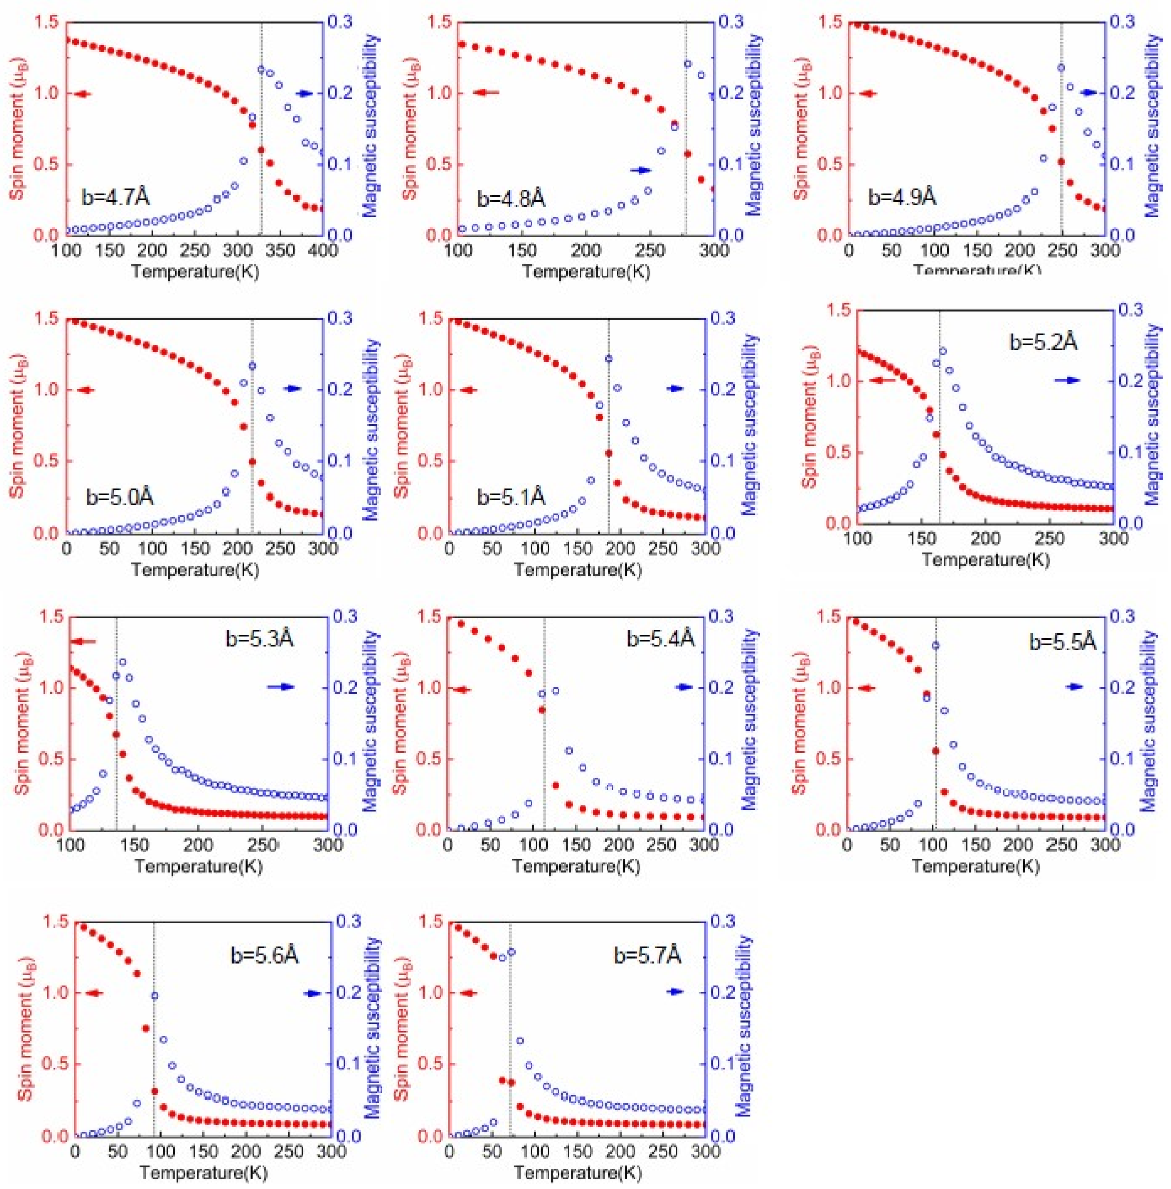


FIG. S15 Average magnetic moment and susceptibility from Monte Carlo simulations for $VGe_2N_4$ under strain.

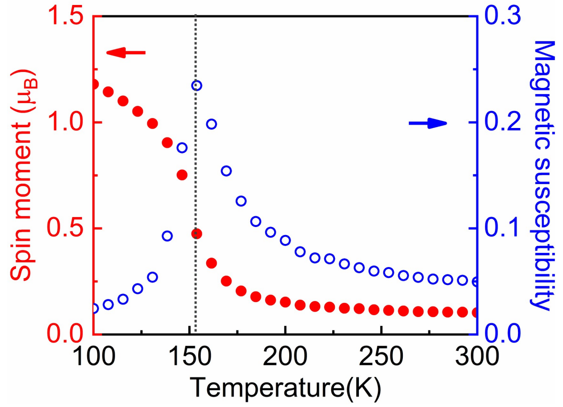


FIG S16 Average magnetic moment and susceptibility from Monte Carlo simulations for $VGe_2N_4$ with anisotropic Heisenberg model.
